# Supplementary material for: Strand plasticity governs fatigue in colloidal gels
Source: arXiv:1709.03286 source file (2017-09-11)
Supplement: Supplementary file 1 [file Supplemental.pdf]

# Supplemental Material to "Strand plasticity governs fatigue in colloidal gels"

Jan Maarten van Doorn,* Joanne E. Verweij,* Joris Sprakel, and Jasper van der Gucht†
*Physical Chemistry and Soft Matter, Wageningen University,*
*Stippeneng 4, 6708 WE, Wageningen, The Netherlands*
(Dated: September 11, 2017)

## SIMULATION DETAILS - MULTIPLE STRAIN AMPLITUDES

A toy model is used to study the effect of repeated deformation on the microscopic scale only. We consider a gel strand with 256 particles which interact through the Morse potential [1]:

$$\beta u(r) = \beta\epsilon \ \exp(\rho_0[a-r]) \ (\exp[\rho_0(a-r)] - 2) \qquad (1)$$

with $\rho_0 = 33$, energy scale $\beta\epsilon = 10$ and particle diameter $a = 2r_a$ (see SI Fig. 1). Individual strands are formed in between two attractive walls ($\rho_0 = 33$, $\beta\epsilon = 10$). The start configuration of these strands is an FCC lattice in a 4 x 4 (height x width) arrangement ($N = 256$). The equilibration time before applying oscillatory deformation is set to $t = 568\ \tau_B$ [2], to make sure that the gel strand can form in between the two attractive walls.

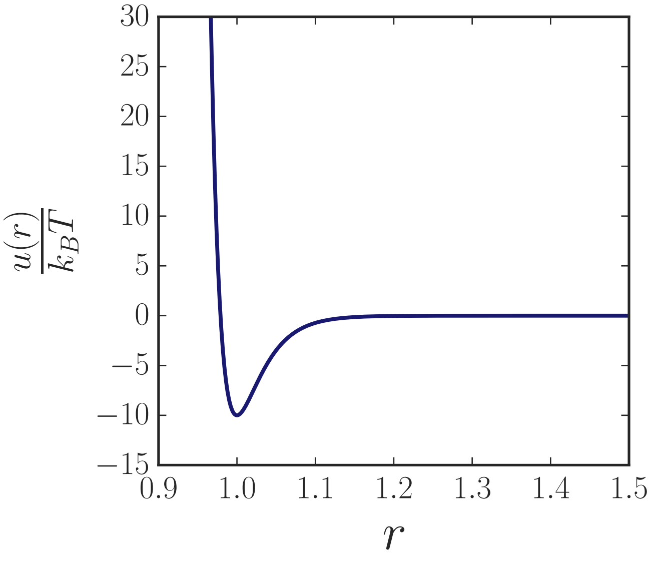


FIG. 1. (color online) Morse potential with interaction range parameter $\rho_0 = 33$ and interaction strength $\beta\epsilon = 10$.

Similar to the experiment, the single gel strand in the BD simulations is cyclically deformed with a sawtooth strain profile (Inset Fig. 4a). One of the walls is moved outward, leding to an expansion at a fixed strain rate $\dot{\gamma} = 0.00284\ \tau_B^{-1}$, with $\tau_B = r_a^2/D$ the self-diffusion time of the particles and $D$ their diffusion coefficient. Note that this strain rate is comparable to a strain rate of $\dot{\gamma} = 6.7\ \mathrm{s}^{-1}$ in the experiment. After 8 successive oscillations the strain amplitude is increased from $\gamma = 0.02$ to $\gamma = 0.04$ and $\gamma = 0.06$ respectively. More than 65 % of the gel strands break after 24 oscillatory expansions at successive strain amplitudes of $\gamma = 0.02, 0.04$ and 0.06.

We note that the fracture of individual strands is highly ductile and occurs by strong necking. Moreover, fracture only occurs when a single bond connects the two halves. In all simulations a percentage of the strands is fractured (either by detaching from the wall or by breaking into clusters, see SI Fig. 6). To focus on plastic mechanisms, data of broken strands is excluded in further analysis. Each strain amplitude contains data of at least 30 statistically different gel strands.

## ANALYSIS - BOND REARRANGEMENTS

To quantify bond rearrangements, we calculate the average fraction of inter-particle bonds that is broken per oscillation cycle:

$$\chi(c_n) = 1 - \langle \frac{n_i(c_n + 1)}{n_i(c_n)} \rangle_p, \qquad (2)$$

where $n_i(c_n)$ is the number of nearest neighbours of particle $i$ at the start of a certain oscillation, $n_i(c_n + 1)$ is the number of these neighbours that remain at the end of this oscillation and the average is taken over all particles $p$ in the strand. We find that the number of broken bonds is highest in the first deformation cycle and decreases gradually (SI Fig. 2b). Similar to previous observations the average number of bonds per particle in the gel strand $N_b$ increases in time (SI Fig. 2c) [3]. Repeated oscillatory deformation hence is reminiscent to activated aging, in which the non-equilibrium gel structure tends to coarsen to increase the number of bonds in the network.

## SIMULATION DETAILS - SINGLE STRAIN AMPLITUDES

For single strain amplitudes simulations are performed exactly such as described in the previous paragraph, however, in this case we do not impose a higher strain

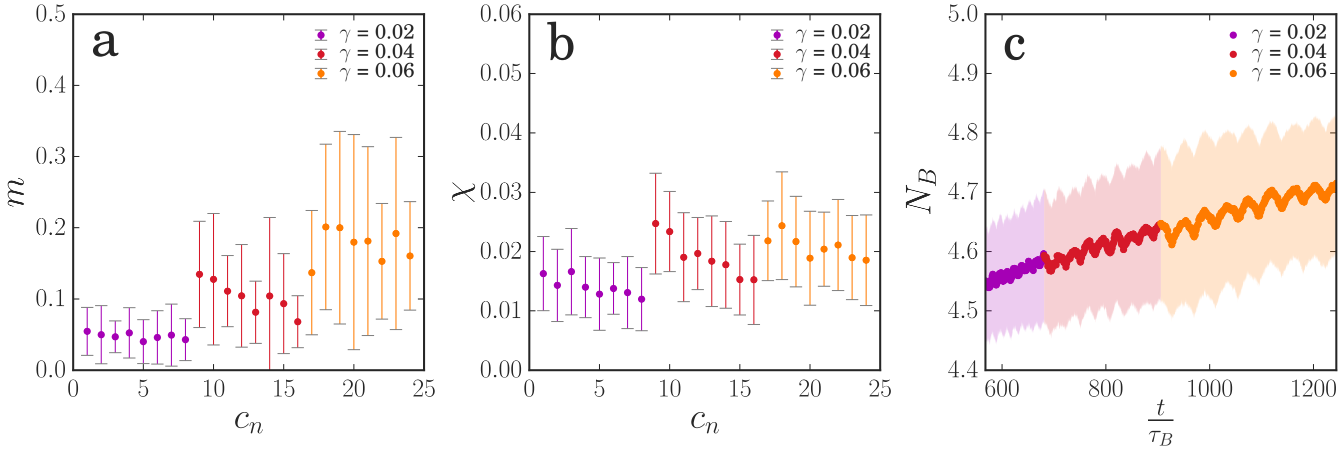


FIG. 2. (color online) (a) Average plastic deformation per oscillation (Eq. q of main text). (b) The fraction of broken bonds per oscillation. (c) Number of bonds in time. The shaded area indicates the variation in the number of bonds between the different strands.

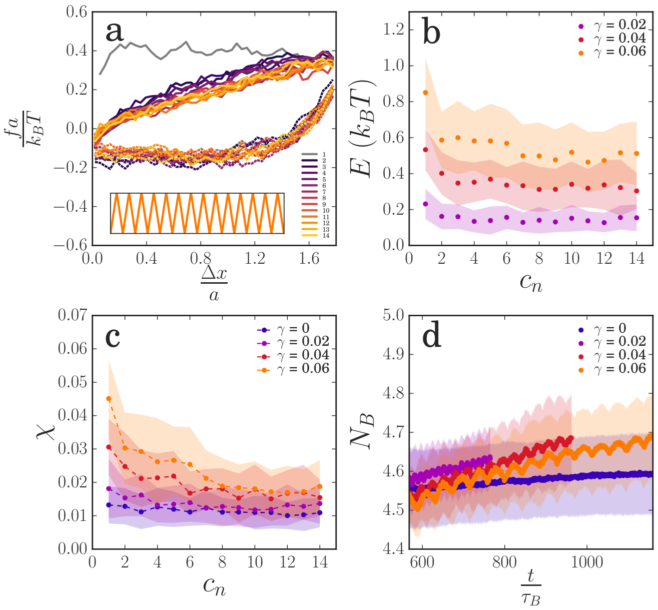


FIG. 3. (color online) (a) Force-distance curve for BD simulations upon 14 oscillatory expansions of a single gel strand at strain amplitude $\gamma = 0.06$. The solid line represents the first part of a single sawtooth, whereas the dotted line indicates the second part. (b) Energy per oscillation for strain amplitudes $\gamma = 0.02$, 0.04 and 0.06 obtained through integration of the force-distance curves. (c) The fraction of bonds that break per oscillation. The dotted line is drawn to guide the eye. (d) Average number of bonds in time. The shaded areas indicate the variation between the different gel strands.

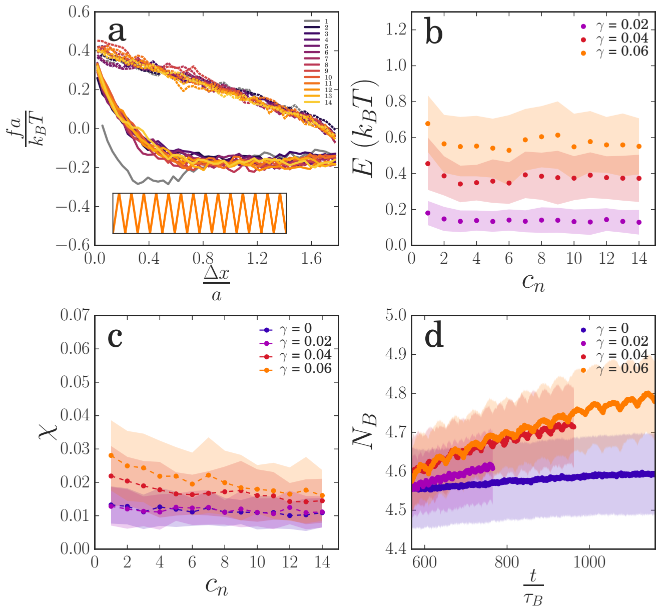


FIG. 4. (color online) Data of BD simulations upon 14 oscillatory compressions of a single gel strand at strain amplitudes $\gamma = 0.02$, 0.04 and 0.06. See SI Fig. 3 for the explanation of each subplot.

after a certain amount of cycles. Data is shown both for expansion (Fig. SI 3) and compression (Fig. SI 4) of single gel strands. In the latter case the distance between the walls is first decreased, leading to compression of the gel strand, after which the walls are brought back to their original position. We impose 14 oscillations in total for strain amplitudes $\gamma = 0.02$, 0.04 and 0.06. The fourth oscillation for these strain amplitudes (expansion) is used to re-scale the force-distance curves as shown in Fig. 4c of the paper.

At higher strain amplitudes compression favours the increase in number of bonds compared to expansion. Both the amount of dissipated energy and the fraction of inter-particle bonds that break per oscillation cycle is lower for compression, i.e. compression enhances the

reformation of inter-particle bonds over expansion.

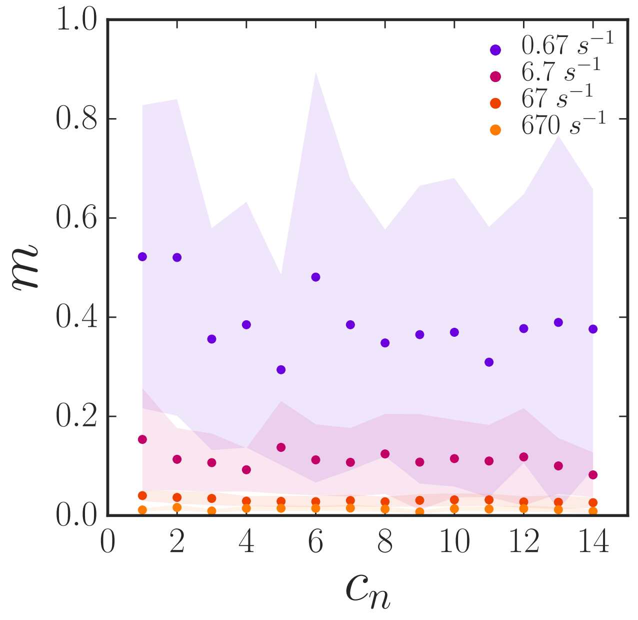


FIG. 5. (color online) Average plastic deformation per oscillation cycle as a function of the strain rate.

## BROKEN GEL STRANDS

Gel strands that break during the simulation are not included in further analysis. Statistics of the broken strands (Fig. SI 6) shows the percentage of strands that detach from the wall or break into clusters. The number of gel strands that break upon expansion is higher compared to compression. Yet, for expansion the majority of the strands break into clusters whereas for compression the effect of breaking at the wall or into clusters is more evenly distributed. Deformation of gel strands at different strain rates $\dot{\gamma}$ only shows different breakage statistics at a strain rate of 670 $s^{-1}$. Here the amount of broken strands increases drastically and strands start to break profoundly at the wall instead of breaking into clusters. This indicates that the amount of broken gel strands is not affected by the strain rate used in the simulations (6.7 $s^{-1}$).


* These authors contributed equally

† jasper.vandergucht@wur.nl



[1] C. P. Royall, J. Eggers, A. Furukawa, and H. Tanaka, Phys. Rev. Lett. **114**, 258302 (2015).

[2] Varying the equilibration time doesn't influence the obtained force-distance curves. However, for too short equilibration times the average number of bonds is still substantially increasing in the zero measurement. See SI Fig. 3 and 4 for the zero measurement (blue curve, $\gamma = 0$) of these simulations.

[3] J. D. Park, K. H. Ahn, and S. J. Lee, Soft Matter **11**, 9262 (2015).

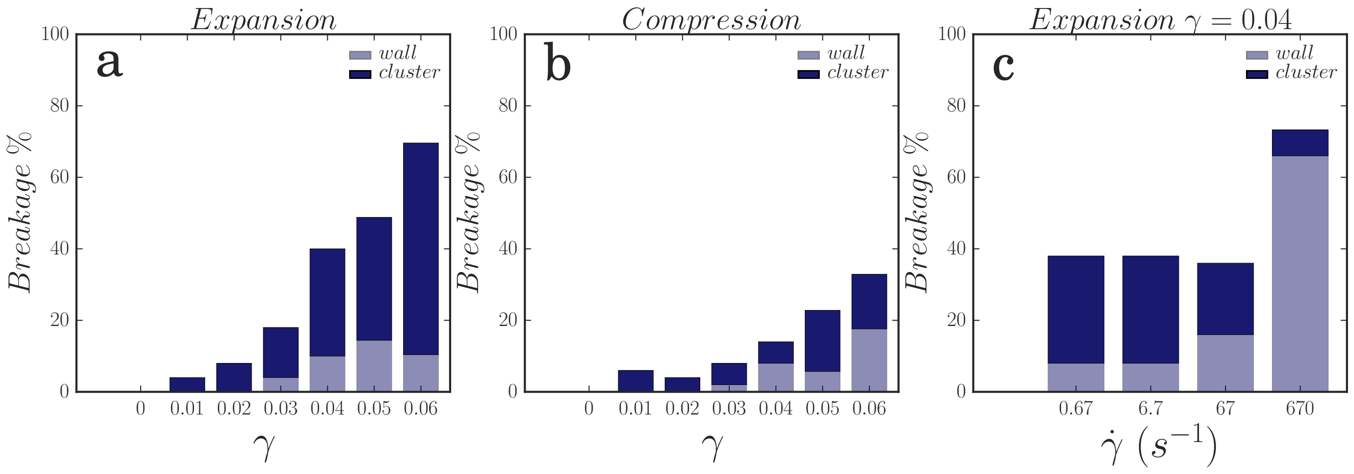


FIG. 6. (color online) Breakage statistics for (a) expansion and (b) compression of gel strands at strain amplitudes $\gamma = 0.01$ - 0.06. (c) Breakage statistics of gel strands that are deformed with strain rates $\dot{\gamma} = 0.67$, 6.7, 67 and 670 $s^{-1}$ respectively (expansion, $\gamma = 0.04$).

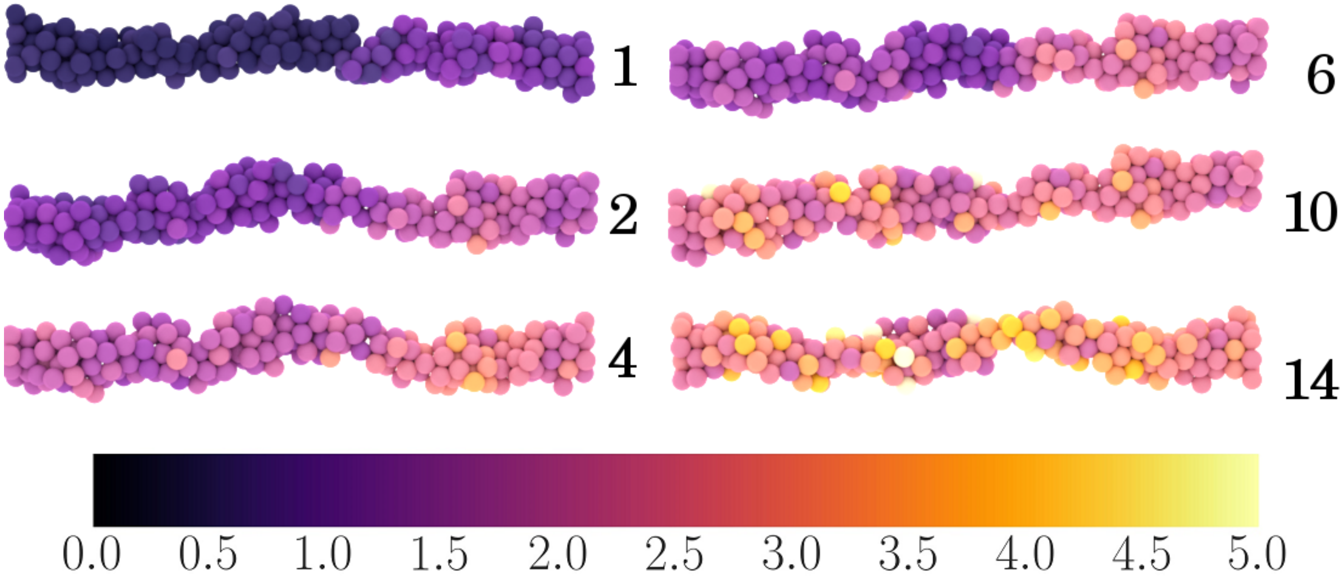


FIG. 7. (color online) Visual representation of the cumulative average plastic deformation in cycles 1,2,4,6,10 and 14 of a single gel strand ($\gamma_{max} = 0.04$). The color bar indicates the cumulative irreversible displacements of the particles from low (purple) to high (yellow).
